# Supplementary material for: A Compressive Sensing Inspired Monte-Carlo Method for Combinatorial Optimization
Source: arXiv:2510.24755 source file (2026-10-29)
Supplement: Supplementary file 1 [file Supplementary_Information.tex]

\documentclass[fleqn,10pt]{wlscirep}
\usepackage[utf8]{inputenc}
\usepackage[T1]{fontenc}

\usepackage{graphicx}
\usepackage{subcaption}
\usepackage[utf8]{inputenc}
\usepackage{dcolumn}
\usepackage{bm}
\usepackage{color}
\usepackage{amsmath} 
\usepackage{physics}
\usepackage{braket}
\usepackage{amssymb}
\usepackage{amsthm}
\usepackage{mathtools} 
\usepackage{amsfonts}
\usepackage{comment}
\usepackage{xcolor}
\usepackage{url}
\usepackage{algorithm}
\usepackage{algorithmic}
\usepackage{soul}
\usepackage{caption}
\usepackage{subcaption}
\usepackage{silence}

\theoremstyle{definition}
\newtheorem{definition}{Definition}
\theoremstyle{definition}

\newtheorem{lemma}{Lemma}

\newtheorem{theorem}{Theorem}
\newtheorem{proposition}{Proposition}

\DeclareMathOperator*{\argmax}{arg\,max}

\captionsetup[table]{name=Supplementary Table}

\title{Supplementary Information}

\author[1,*]{Baptiste Chevalier}
\author[1]{Shimpei Yamaguchi}
\author[1]{Wojciech Roga}
\author[1,2]{Masahiro Takeoka}
\affil[1]{Department of Electronics and Electrical Engineering, Keio University, Yokohama 223-8522, Japan}
\affil[2]{Advanced ICT Research Institute, National Institute of Information and Communications Technology (NICT), Koganei, Tokyo 184-8795, Japan}

\affil[*]{chevalier.baptiste@keio.jp}

%\keywords{Keyword1, Keyword2, Keyword3}

\begin{abstract}
In this Supplementary Information, we present supplementary properties of the mathematical objects used in the main text. We also provide a detailed discussion and intuition regarding the MCCO algorithm applied to a simplified interpretable example, and provide proofs of less important quantities which appear in the main text. These materials are not crucial to the main text; however, they provide additional insight into the mechanism of the algorithm and the meaning and relevance of the functions used in numerical simulations. 

In Supplementary Information 1, we discuss some notable properties of the transform from the small set of rules to the large scale compressible functions. Such a function is introduced in the Methods and used in numerical simulations. It can be interpreted as a large scale code that embeds the rules. We prove properties such as injectivity, properties of the norm, and distances. 

In Supplementary Information 2, we discuss the coherence we mentioned in the Theoretical analysis. We give a formal expression for the coherence of structured matrices that were used in the numerical simulations of the paper. 

In Supplementary Information 3, we discuss the effect of thresholding on the variance of the objective function and its importance in the MCCO algorithm. 

Finally, in Supplementary Information 4, we discuss a simple example that explains working of MCCO algorithm. The example shows how the solution of Problem II can be reduced to the solution of Problem I. This specific example uses a structured matrix acting on nearest neighbor pairs of bits and we interpret sketch functions as correlations that can be extracted from the samples.\\

The notations used in this document are the same as in the main text, refer to the paper for definitions.

\end{abstract}
\begin{document}

\flushbottom
\maketitle

\thispagestyle{empty}

\section{Properties of the $F_N$ transform}
\label{app:transform_prop}

\subsection{Properties}

\noindent The proofs follow the list of statements.

\begin{theorem}
	\label{cl:prop}
	Given a string $a$ (a rule) of size $k$:
	\begin{enumerate}
		\item $\|F_N(a)\|\geq 0$.
		\item $F_k = id$   (if $n=k$, the transform is the identity), i.e., $F_k(a)=\bf{a}$.
		\item $F_N$ can be written as a $2^N \times 2^k$ rectangular matrix.
	\end{enumerate}
\end{theorem}
\noindent The proofs of Theorem \ref{cl:prop} are trivial. 

\begin{theorem}{[Injectivity]}
	\label{theo:inject}
	\begin{equation}
		F_N(a)=F_N(b) \iff a=b .
	\end{equation} 
\end{theorem}

\begin{definition}{[$\ell_1$-Norm of the transform]}
	\begin{equation} \|F_N(a)\|_1=\sum_{x\in\lbrace0,1\rbrace^N}\sum_{i=1}^{N-k+1} \delta_{h(x_i,a),0}.
	\end{equation}
\end{definition}

\begin{theorem}{[$\ell_1$-Norm Recursive Expression]}
	\label{theo:normrec}
	\begin{equation}
		\|F_{N+1}(a)\|_1=2 \|F_N(a)\|_1 +2^{N-k+1}.
	\end{equation}
\end{theorem}

\begin{theorem}{[$\ell_1$-Norm Explicit Expression]}
	\label{theo:norm}
	\begin{equation}
		\|F_{k+l}(a)\|_1=2^l(l+1).
	\end{equation}
	Notice that all elements $a$ have the same norm!
\end{theorem}

\begin{theorem}{[Rules separations]}
	\label{theo:rule_dist}
	
	For any $a,b\neq a\in\{0,1\}^k$ and for any $d\geq0$, there exists $N$ such that
	$$
	\|F_N(a)-F_N(b)\|_2\geq d.
	$$
\end{theorem}

\begin{theorem}{[Moments arbitrary distance]}
	\label{theo:moment_dist}
	
	Let $\Phi : \mathbb{R}^{2^N} \rightarrow \mathbb{R}^{M}$ be a map computing $M$ generalized moments of the function $\pi$ whose density is $f_{\mathcal{R}}$. The sketch map $\Phi \in \mathbb{R}^{2^N \times M}$ is chosen as a typical compressive sensing map (with RIP or random projections).
	For any $a,b\neq a\in\{0,1\}^k$ and for any $D\geq0$, there exists $N$ such that:
	\begin{equation}
		\label{eq:tp}
		\| \Phi(F_N(a)) - \Phi(F_N(b)) \|_2 \geq D.
	\end{equation}
\end{theorem}

\subsection{Proofs or the above properties\\}

\begin{lemma}{prerequisite for Theorem \ref{theo:inject}}
	\label{lem:1}
	\begin{equation}
		a\neq 0^{(k)}\implies F_N(a)[i_a]=1.
	\end{equation} 
\end{lemma}
\begin{proof}
	The proof is by contradiction.\\
	$a=a_1\cdots a_k$ matches with $i_a=0^{(N-k)}a_1\cdots a_k$ at the last $k$ bits.
	If we assume $F_N(a)[i_a]>1$, then, $a$ matches with $i_a$ at somewhere else, say $a_1\cdots a_k=0^{(l)}a_1\cdots a_{k-l}, (l\in\mathbb{Z}^{+}, 1\leq l\leq k-1)$.
	Then we get $a=0^{(k)}$ by solving
	\begin{align*}
		a_1&=0,\\
		&\ \ \vdots \\
		a_{l}&=0,\\
		a_{l+1}&=a_1,\\
		&\ \ \vdots \\
		a_{k}&=a_{k-l}.
	\end{align*}
	This contradicts with $a\neq 0^{(k)}$.
\end{proof}

\begin{proof}{of Theorem \ref{theo:inject}}
	
	The proof that $a=b \implies F_N(a)=F_N(b)$ : is trivial from the definition of $F_N$. Thus we only need to prove $F_N(a)=F_N(b) \implies a=b$. To do so, we use the contraposition that is, we want to prove that $a \neq b \Longrightarrow F_N(a)\neq F_N(b).$\\
	Set
	\begin{align*}
		&a=a_1\cdots a_k, (a_i\in\lbrace 0,1\rbrace, i=1,\cdots k),\\
		&b=b_1\cdots b_k, (b\in\lbrace 0,1\rbrace, i=1,\cdots k),\\
		&0^{(m)}=\underbrace{0\cdots 0}_{m},\\
		&i_a=0^{(N-k)}a_1\cdots a_k,\\
		&i_b=0^{(N-k)}b_1\cdots b_k,
	\end{align*}
	and $F_N(a)[i]$ where $i\in\lbrace0,1\rbrace^n$ denotes the $i$-th element of the vector $F_N(a)$.\\\\
	Case i) When $a=0^{(k)}$\\
	$F_N(a)[0^{(N)}]=N-k+1$, by the definition of $F_N$.
	$F_N(b)[0^{(N)}]=0$, since $b\neq a=0^{(k)}$.
	Thus, $F_N(a)\neq F_N(b)$.\\
	\\
	Case ii) When $a\neq 0^{(k)}$\\
	Let $b\neq 0^{(k)}$, since the case of $b=0^{(k)}$ can be proved completely the same as the case of $a=0^{(k)}$. We prove by contradiction. Assume $F_N(a)=F_N(b)$.
	This gives
	\begin{align}
		F_N(a)[i_a]&=F_N(b)[i_a],\label{eq:ia}\\
		F_N(a)[i_b]&=F_N(b)[i_b].\label{eq:ib}
	\end{align}
	From Lemma \ref{lem:1} and equation \eqref{eq:ia}, $F_N(b)[i_a]=1$. Thus, for an integer $k_1,\ 1\leq k_1\leq k-1$,
	\begin{equation}
		b_1\cdots b_k=0^{(k_1)}a_1\cdots a_{k-k_1}\label{eq:b}
	\end{equation}
	since $0\neq b\neq a$.\\
	From Lemma \ref{lem:1} and equation \eqref{eq:ib}, $F_N(a)[i_b]=1$. Thus, for an integer $k_2,\ 1\leq k_2\leq k-1$,
	\begin{align*}
		a_1\cdots a_k&=0^{(k_2)}b_1\cdots b_{k-k_2}\\
		&= 
		\begin{cases}
			0^{(k_2)}0^{(k_1)}a_1\cdots a_{k-k_1-k_2} & \text{if $k-k_2\geq k_1+1$} \\
			0^{(k_2)}0^{(k-k_2)} & \text{if $k-k_2\leq k_1$} 
		\end{cases}
	\end{align*}
	by equation \eqref{eq:b} and $0\neq a\neq b$ . By considering the same way in the proof of Lemma \ref{lem:1}, $a$ will be $0^{(k)}$ in both cases. This contradicts with $a\neq 0^{(k)}$. Therefore, $F_N(a)\neq F_N(b)$.    
\end{proof}

\begin{lemma}{prerequisite for Theorem \ref{theo:normrec}}
	\label{lem:2}
	\begin{align*}
		F_{N+1}(a)&=
		\begin{pmatrix}
			F_N(a)\\
			F_N(a)
		\end{pmatrix}
		+\bf{a}\otimes \mathbf{1}_{2^{N-k+1}}\\
		&=\mathbf{1}_{2}\otimes F_N(a)+\bf{a}\otimes \mathbf{1}_{2^{N-k+1}},
	\end{align*} 
	where $\otimes$ is the tensor product, $\mathbf{1}_n$ denotes $n$ length column vector with all elements $1$, and $\bf{a}$ is the $2^k$-length column vector of which $a$-th element is $1$ and the rest is $0$.
\end{lemma}

\begin{proof}
	An $(N+1)$-bit string $x^{(N+1)}\in\lbrace0,1\rbrace^{N+1}$ can be made by putting $0$ or $1$ in front of an $N$-bit string $x^{(N)}\in\lbrace 0,1\rbrace^N$. 
	We can divide $\lbrace 0,1\rbrace^N$ into two sets: a set $X$ which consists of $N$-bit strings which start with $(k-1)$ bits matching the $(k-1)$ last bits of $a$, i.e. $a_2\cdots a_k$ and its complementary set $\bar{X}$ made of the remaining $N$-bit strings.
	Put $a_1$ in front of $x^{(N)}\in X$ and generate $(N+1)$-bit string $a_1x^{(N)}$. Then the number of $k$-bit strings in $a_1x^{(N)}$  that matches with $a$ increases by one from the number of $k$-bit strings in $x^{(N)}$  that matches with $a$, because $x^{(N)}\in X$ starts with $a_2\cdots a_k$. In other cases, i.e., 
	\begin{enumerate}
		\item[$\cdot$] putting $1 - a_1$ in front of $x^{(n)}\in X$ and
		\item[$\cdot$] putting $a_1$ or $1 -^ a_1$ in front of $x^{(n)}\in \bar{X}$,
	\end{enumerate}
	the number of $k$-bit strings that matches with $a$ does not change. Writing this explicitly,
	\begin{equation*}
		F_{N+1}(a)[yx^{(N)}]=
		\begin{cases}
			F_N(a)[x^{(N)}]+1 &\text{if $y=a_1 \land x^{(N)}\in X$},\\
			F_N(a)[x^{(N)}] &\text{else}.
		\end{cases}
	\end{equation*}
	Therefore, we can calculate $F_{N+1}(a)$ by the following procedure;
	\begin{enumerate}
		\item Concatenate $F_N(a)$ and $F_N(a)$,
		\item Add 1 to the elements of which indexes start from $k$-bit string $a$.
	\end{enumerate}
	The $2^{N+1}$ length vector indicating the position of $(N+1)$-bit strings which start from $a$ can be written as $\bf{a}\otimes \mathbf{1}_{2^{N-k+1}}$, since there are $2^{N+1-k}$ strings like that. Thus, the equation in Lemma \ref{lem:2} holds.
\end{proof}

\begin{proof}{of Theorem \ref{theo:normrec}}
	By taking the $\ell_1$-norm on each side of the equation from Lemma \ref{lem:2}, it can easily be shown. (both vectors on the right hand side of the equation are vectors with non-negative elements.)
\end{proof}

\begin{proof}{of Theorem \ref{theo:norm}\\}
	By substituting $N$ in Theorem \ref{theo:normrec} to $k+l$,
	\begin{equation*}
		\|F_{k+l+1}(a)\|_1=2\|F_{k+l}(a)\|_1+2^{l+1}.
	\end{equation*}
	Set $\|F_{k+l}(a)\|_1=s_l$. Then,
	\begin{align*}
		s_{l+1}&=2s_l+2^{l+1},\\
		\dfrac{s_{l+1}}{2^{l+1}}&=\dfrac{s_l}{2^{l}}+1.
	\end{align*}
	Thus, 
	\begin{align*}
		\dfrac{s_l}{2^l}&=\dfrac{s_0}{2^0}+l,\\
		\dfrac{s_l}{2^l}&=1+l, \quad(\because s_0=\|F_k(a)\|_1=\|\bf{a}\|_1=1)\\
		\|F_{k+l}(a)\|_1&=s_l\\
		&=2^{l}(l+1).
	\end{align*}
\end{proof}

\begin{lemma}{prerequisite for Theorem \ref{theo:rule_dist}\\}
	\label{lem:l2_diff}
	When $a\neq b$,
	\begin{align*}
		&\|F_{k+l}(a)-F_{k+l}(b)\|_2^2\\
		\geq&
		\begin{cases}
			2^{l+1}\left(\dfrac{3}{5}l-\dfrac{1}{9}-\dfrac{\frac{4}{3}k+\frac{2}{3}l+\frac{20}{9}}{2^{k-2}}\right) & (k:\text{even})\\
			2^{l+1}\left(\dfrac{3}{5}l-\dfrac{1}{9}-\dfrac{\frac{5}{3}k+\frac{1}{3}l+\frac{16}{9}}{2^{k-2}}\right) & (k:\text{odd}).
		\end{cases}
	\end{align*}
\end{lemma}

\begin{proof}{ of Lemma \ref{lem:l2_diff}}
	\begin{align*}
		&\|F_N(a)-F_N(b)\|_2^2\\
		=&F_N(a)\cdot F_N(a)+F_N(b)\cdot F_N(b)-2F_N(a)\cdot F_N(b)
	\end{align*}
	Thus, we will analyze $F_N(a)\cdot F_N(b)$.
	From
	\begin{equation*}
		F_{k+l}(a)=\sum_{i=1}^{l+1}\left(\bm{1}_2^{\otimes (i-1)}\otimes\ket{a}\otimes\bm{1}_2^{\otimes (l+1-i)} \right),
	\end{equation*}
	the inner product becomes
	\begin{align*}
		&F_{k+l}(a)\cdot F_{k+l}(b) \\
		=& \sum_{i=1}^{l+1}\left(\mathbf{1}_2^{\otimes (i-1)}\otimes\ket{a}\otimes\mathbf{1}_{2}^{\otimes (l+1-i)} \right)^{\mathsf{T}}\\ &\quad \quad \sum_{i^{\prime}=1}^{l+1}\left(\mathbf{1}_2^{\otimes (i^{\prime}-1)}\otimes\ket{b}\otimes\mathbf{1}_{2}^{\otimes (l+1-i^{\prime})} \right)\\
		=&\sum_{i=i^{\prime}}\left(\mathbf{1}_2^{\otimes (i-1)}\otimes\ket{a}\otimes\mathbf{1}_{2}^{\otimes (l+1-i)} \right)^{\mathsf{T}}\\
		&\quad \quad\left(\mathbf{1}_2^{\otimes (i^{\prime}-1)}\otimes\ket{b}\otimes\mathbf{1}_{2}^{\otimes (l+1-i^{\prime})} \right)\\
		+&\sum_{i\neq i^{\prime}}\left(\mathbf{1}_2^{\otimes (i-1)}\otimes\ket{a}\otimes\mathbf{1}_{2}^{\otimes (l+1-i)} \right)^{\mathsf{T}}\\ &\quad \quad \left(\mathbf{1}_2^{\otimes (i^{\prime}-1)}\otimes\ket{b}\otimes\mathbf{1}_{2}^{\otimes (l+1-i^{\prime})} \right).
	\end{align*}
	For the first term,
	\begin{align*}
		&\sum_{i=i^{\prime}}\left(\mathbf{1}_2^{\otimes (i-1)}\otimes\ket{a}\otimes\mathbf{1}_{2}^{\otimes (l+1-i)} \right)^{\mathsf{T}}\\&\quad \quad\left(\mathbf{1}_2^{\otimes (i^{\prime}-1)}\otimes\ket{b}\otimes\mathbf{1}_{2}^{\otimes (l+1-i^{\prime})} \right)\\
		=&\sum_{i=1}^{l+1} \left(\mathbf{1}_2^{\otimes(i-1)\mathsf{T}}\mathbf{1}_2^{\otimes(i-1)}\right)\braket{a|b}\left(\mathbf{1}_{2}^{\otimes (l+1-i)\mathsf{T}}\mathbf{1}_{2}^{\otimes (l+1-i)}\right)\\
		=& \begin{cases}
			0 & (a\neq b)\\
			(l+1)2^{l} &(a=b)
		\end{cases},
	\end{align*}
	since $\braket{a|b}=\delta_{a,b}$.\\
	For the second term with $a\neq b$, the positions of $\ket{a}$ and $\ket{b}$ differ, so the calculation of the inner product will not be easy as the case of the first term. Here we assume that $l\geq k$ and will divide the second term into two cases; (i) when the positions of $\ket{a}$ and $\ket{b}$ do not overlap, and (ii) when they overlap. The case of $l<k$ can be regarded as only considering Case (ii).\\
	Case i): when the positions of $\ket{a}$ and $\ket{b}$ do not overlap\\
	It can be illustrated as $(l-k+1)$ cases shown below (there are $\mathbf{1}_2$s in the blank places):  
	\begin{align*}
		a_1a_2\cdots a_{k-1}a_{k}&\\
		&b_1b_2\cdots b_{k-1}b_{k},\\
		\\
		a_1a_2\cdots a_{k-1}a_{k}&\\
		&\underbrace{}_{1}b_1b_2\cdots b_{k-1}b_{k},\\
		\\
		a_1a_2\cdots a_{k-1}a_{k}&\\
		&\underbrace{\quad\quad}_{2}b_1b_2\cdots b_{k-1}b_{k},\\
		\vdots\\
		\vdots\\
		a_1a_2\cdots a_{k-1}a_{k}&\\
		&\underbrace{\quad\quad\quad\quad}_{l-k} b_1b_2\cdots b_{k-1}b_{k}.
	\end{align*}
	Here I showed the case when $a_k$ is in front of $b_1$. The opposite case (when $b_k$ is in front of $a_1$) can be considered in the completely same way. For all of them, the inner product will be $2^{l-k}$, because the inner product of $\ket{a_i}$ (or $\ket{b_i}$) and $\mathbf{1}_2$ will be $1$ for all $1\leq i\leq k$ (there are $2k$ of this inner products), and the inner product of $\mathbf{1}_2$ and $\mathbf{1}_2$ will be $2$ (there are $(l-k)$ of this inner product).  When there is $g$-length gap between the positions of $a_k$ and $b_1$, there are $(l-k-g+1)$ options for the position of $a_1$.  Thus, the sum of inner products is
	\begin{equation*}
		2\cdot2^{l-k}\sum_{g=0}^{l-k}(l-k-g+1)=2^{l-k}(l-k+1)(l-k+2).
	\end{equation*}
	Case ii): when the position of $\ket{a}$ overlaps with the position of $\ket{b}$\\
	These cases will be illustrated as below; when $a_1$ is in front of $b_1$ (Case ii-1)
	\begin{align*}
		&a_1a_2\cdots a_{k-1}a_{k}\\
		&\quad b_1b_2\cdots\quad\ b_{k-1}b_{k},\\
		\\
		&a_1a_2a_3\cdots a_{k-1}a_{k}\\
		&\quad \quad b_1b_2\cdots\quad b_{k-2}b_{k-1}b_{k},\\
		\vdots\\
		\vdots\\
		&a_1a_2\cdots a_{k-1}a_{k}\\
		&\quad \quad \quad\quad\quad\,\,\, b_1b_2\cdots b_{k-1}b_{k},
	\end{align*}
	and when $b_1$ is in front of $a_1$ (Case ii-2)
	\begin{align*}
		&\quad a_1a_2\quad\cdots\quad a_{k-1}a_{k}\\
		&b_1b_2\cdots\quad\ b_{k-1}b_{k},\\
		\\
		&\quad\,\,\,\, a_1a_2a_3\cdots a_{k-2}a_{k-1}a_{k}\\
		&b_1b_2b_3\quad\cdots\quad b_{k},\\
		\vdots\\
		\vdots\\
		&\quad \quad \quad\quad\quad a_1a_2\cdots a_{k-1}a_{k}\\
		&b_1b_2\cdots b_{k-1}b_{k}.
	\end{align*}
	For both (Case ii-1) and (Case ii-2) the $j$th pattern represents the case when the positions of $a_1$ and $b_1$ are $j$-separated. For $j$-separated case, the sum of the inner product is 
	\begin{equation*}
		\begin{cases}
			(l-j+1)2^{l-j} &\text{when overlapping part of $a$ and $b$ is same},\\
			0 &\text{else}.
		\end{cases}
	\end{equation*}
	This value depends on $a$ and $b$. We will calculate the maximum value of the inner product of this part. The task is to find the possible combination which gives the maximum inner product value from the below table.
	\renewcommand{\arraystretch}{1.5}
	\begin{table}[H]
		\centering
		\begin{tabular}{|c|c|c|}\hline
			$j$ & Case ii-1 & Case ii-2  \\ \hline\hline
			$1$ & $l2^{l-1}$ & $l2^{l-1}$ \\ \hline
			$2$ & $(l-1)2^{l-2}$ & $(l-1)2^{l-2}$ \\ \hline
			$\vdots$ & $\vdots$ & $\vdots$ \\ \hline
			$k-1$ & $(l-k+2)2^{l-k+1}$ & $(l-k+2)2^{l-k+1}$ \\ \hline
		\end{tabular}
		\caption{Maximum inner product value for each separation value $j$}
		\label{tb:Case-ii}
	\end{table}
	\renewcommand{\arraystretch}{1.0}
	First, choose $l2^{l-1}$ and $l2^{l-1}$. This is because 
	\begin{align*}
		&(l-1)2^{l-2}+\cdots+(l-k+2)2^{l-k+1}\\
		=&\sum_{j=2}^{k-1}(l-j+1)2^{l-j}\\
		=&2^{l-1}\left[l-2-\left(\dfrac{1}{2}\right)^{k-2}(k+l+2)\right]\\
		\leq& 2^{l-1}l,
	\end{align*}
	so you get more than half of the possible inner product value by choosing them. If you choose these two, $a_2\cdots a_k=b_1\cdots b_{k-1}$ and $a_1\cdots a_{k-1}=b_2\cdots b_k$ have to be simultaneously held. You can easily see that this condition gives
	\begin{align*}
		a=01010101\cdots\\
		b=10101010\cdots
	\end{align*}
	or the opposite. This also satisfies the conditions for $j$: odd. You can see it by sliding $a$ (or $b$) to the right for $j$: odd positions. If you try to satisfy any of the condition for $j$: even for the above $a$ and $b$, it will immediately gives you $a=b=0000\cdots (\text{or}\ 1111\cdots)$.\\
	Finally, the maximum inner product value for case (ii) is
	\begin{align*}
		&2\sum_{j: \text{ odd}}(l-j+1)2^{l-j}\\
		=&
		\begin{cases}
			2\sum_{m=1}^{n}\left[l-(2m-1)+1\right]2^{l-(2m-1)}&(k=2n)\\
			2\sum_{m=1}^{n-1}\left[l-(2m-1)+1\right]2^{l-(2m-1)}&(k=2n-1)
		\end{cases}\\
		=&
		\begin{cases}
			\dfrac{2^{l+2}}{9}\left[3l-2+\dfrac{6n-3l+2}{4^n}\right]\\
			\dfrac{2^{l+2}}{9}\left[3l-2+\dfrac{6n-3l-4}{4^{n-1}}\right]
		\end{cases}\\
		=&
		\begin{cases}
			\dfrac{2^{l+2}}{9}\left[3l-2+\dfrac{3k-3l+2}{2^k}\right]&(k:\text{even})\\
			\dfrac{2^{l+2}}{9}\left[3l-2+\dfrac{3k-3l-1}{2^{k-1}}\right]&(k:\text{odd}).
		\end{cases}
	\end{align*}
	For the second term with $a=b$, the sum of inner product value will be the sum of
	\begin{equation*}
		2^{l-k}(l-k+1)(l-k+2)
	\end{equation*}
	which is from Case (i) and 
	\begin{equation*}
		2\sum_{j=1}^{k-1}(l-j+1)2^{l-j}=2^l\left[2l-2-\left(\dfrac{1}{2}\right)^{k-2}(k+l+2)\right]
	\end{equation*}
	which is the sum of all the values in TABLE~\ref{tb:Case-ii} from Case (ii). We also observe that $F_N(a)\cdot F_N(a)$ does not depend on $a$. Thus, we can rewrite $\|F_N(a)-F_N(b)\|_2^2$ as
	\begin{equation*}
		\|F_N(a)-F_N(b)\|_2^2=2[F_N(a)\cdot F_N(a)-F_N(a)\cdot F_N(b)].
	\end{equation*}
	Therefore we have to check the difference between $F_N(a)\cdot F_N(a)$ and $F_N(a)\cdot F_N(b)$. For the first term, the difference is $(l+1)2^l$. For the second term, the difference appears in Case (ii), and the minimum difference is
	\begin{align*}
		&2^l\left[2l-2-\left(\dfrac{1}{2}\right)^{k-2}(k+l+2)\right]\\
		-&
		\begin{cases}
			\dfrac{2^{l+2}}{9}\left[3l-2+\dfrac{3k-3l+2}{2^k}\right]&(k:\text{even})\\
			\dfrac{2^{l+2}}{9}\left[3l-2+\dfrac{3k-3l-1}{2^{k-1}}\right]&(k:\text{odd}).
		\end{cases}
	\end{align*}
	Add these differences and double it, and we get Lemma \ref{lem:l2_diff}.
\end{proof}

\begin{proof}{ of Theorem \ref{theo:rule_dist}}
	We combine both previous lemmas. Lemma \ref{lem:l2_diff} tells us that the distance between $a$ and $b$ increases exponentially when $N$ grows. Thus, for any $d\geq0$, there exists $N$ such that $\|F_N(a)-F_N(b)\|_2 \geq d$.
\end{proof}

\begin{proof}{ of Theorem \ref{theo:moment_dist}}
	
	According to the Johnson-Lindenstrauss lemma, we have:
	\begin{align*}
		(1- \delta) \|F_N(a) - F_N(b) \|_2 &\leq \|\Phi(F_N(a) - F_N(b)) \|_2 \\ &\leq (1+\delta) \|F_N(a) - F_N(b) \|_2,
	\end{align*}
	where $\delta \in [0,1]$ is a constant and for a number of measurements scaling as $M = O(\frac{k}{\delta^2})$.
	In particular:
	\begin{equation*}
		\|F_N(a) - F_N(b) \|_2 \leq \frac1{1 - \delta} \|\Phi(F_N(a) - F_N(b)) \|_2.
	\end{equation*}
	
	\noindent However, from Theorem \ref{theo:rule_dist} we know that there exists N such that:
	\begin{equation*}
		d \leq \|F_N(a) - F_N(b) \|_2,
	\end{equation*}
	for any $d$.
	And so, for the same $N$, and because $\Phi$ is linear:
	\begin{align*}
		d(1-\delta) \leq \|\Phi(F_N(a)) - \Phi(F_N(b)) \|_2.
	\end{align*}
	Because this holds for any $d$, one just need to chose it in such a way that $d \geq D/(1-\delta)$ to get the desired property.
\end{proof}

\newpage
\section{Coherence of structured matrices}
\label{app:coherence}

\begin{theorem}
	The coherence of a structured matrix using nearest-neighbor patterns of size $k$ acting on a space of $N$ bits is given by
	$$
	\mu = \frac{N-k}{N-k+1}.
	$$
\end{theorem}
\begin{proof}
	The $k$-uplet can be positioned starting from $N-(k-1)$ distinct positions (e.g. $N-1$ for pairs, $N-2$ for triplets etc…).
	
	So any column of the structured matrix has $N-k+1$ entries and the associated normalization factor is $\frac1{\sqrt{N-k+1}}$.
	
	Then for each of the $N-k+1$ starting position, the first column matches with the second column except for the last position, i.e. when we look at each bit individually.
	
	The number of match which contribute to the scalar product is then $N-k$.
\end{proof}

\begin{theorem}
	The coherence of a structured matrix using all possible patterns of size $k$ acting on a space of $N$ bits is given by
	$$
	\mu = \frac{\binom{k}{N-1}}{\binom{k}{N}}.
	$$
\end{theorem}
\begin{proof}
	For full matrices we can place the measured $k$-uplet at $\binom{k}{N}$ starting positions.
	
	So any column of the structured matrix has $\binom{k}{N}$ entries and the normalization factor is $\frac1{\sqrt{\binom{k}{N}}}$.
	
	Then for each of the $\binom{k}{N}$ starting position, the first column matches each time with the second column except when one of the measured bit is in last position, i.e. when we look at each bit individually.
	
	The number of case where this does not happened is exactly $\binom{k}{N-1}$.
\end{proof}

\newpage
\section{Effect of Thresholding}
\label{app:stability_uniqueness}

We can show that a clever use of thresholding usually results in lowering the variance.

We define $T_t$ the thresholding operator which sets every value lower than 
$t$ to $0$, i.e. 
$$
T_t : x \mapsto \begin{cases}
	x \text{ if } x\geq t\\
	0 \text{ else}
\end{cases}.
$$

\begin{theorem}{[Threshold increases probabilities]}
	\label{theo:thresh_impr}
	
	Let $\sigma^{(t)^2} = \text{Var}[\Phi(T_tf_{\mathcal{R}}(x))]$ be the variance of the thresholded function. Recall, $\sigma^2$ is the variance of the original function $f_{\mathcal{R}}$.
	
	There exists a value $t$ for the thresholding parameter for which the variance decreases:	              \begin{equation}
		\label{eq:sigma_ineq}
		\sigma^{(t)^2} \leq \sigma^2.
	\end{equation}
\end{theorem}
The following lemma is used for the proof.

\begin{lemma}{[Concentration Bound with Thresholding]}
	\label{lem:concentration_bound}
	
	Let $\sigma^{(t)^2} = \text{Var}[\Phi(T_tf_{\mathcal{R}}(x))]$ be the variance of the thresholded function. The following expression holds: 
	\begin{equation}
		\sigma^{(t)^2} = p(t) \sigma_1^2(t) + \mu_1^2(t)(1-p(t)p(t) ,
	\end{equation}
	where $p(t)$ is the probability to sample from the non-zero region of $T_tf_{\mathcal{R}}$ after thresholding, $\mu_1$ and $\sigma_1^2$ are respectively the mean and variance of this non-zero region.
\end{lemma}

\begin{proof}
	To express $\sigma^{(t)^2}$ we use the law of total variance. For a given $t$, let's divide the space of $\Phi(T_t f_{\mathcal{R}}(x))$ into its zero part ($G=0)$ and its non-zero part ($G=1)$. The law of total variance allows us to write the variance $\text{Var}[\Phi(T_t f_{\mathcal{R}}(x))]$ (which we will call $\text{Var}(X)$ for convenience) as follows:
	$$
	\text{Var}(X) = \mathbb{E}[\text{Var}[X|G]] + \text{Var}[\mathbb{E}[X|G]],
	$$
	where $G$ is our grouping variable separating the zero part from the non-zero part.
	Assume 
	\begin{itemize}
		\item $\mu_0=0$,\quad $\sigma_0=0$.
		\item $\mu_1$, \quad$\sigma_1$
	\end{itemize}
	are the mean and variance of respectively the zero and non-zero parts.
	The first term of $\text{Var}(X)$ (within group variance) turns into $\mathbb{E}[\text{Var}[X|G]] = p_1 \sigma_1^2$.
	
	The second term (between group variance) can be computed as well:
	we have $\mu = p_0\mu_0+p_1\mu_1$ for the total mean
	\begin{align*}
		\text{Var}[\mathbb{E}[X|G]] &= p_0(\mu_0-\mu)+p_1(\mu_1-\mu)\\
		&= p_0(\mu_0-\mu)+p_1(\mu_1-\mu) \\
		&= p_0\mu_1^2p_1^2 + p_1\mu_1^2(1-p_1)^2\\
		&=\mu_1^2p_0p_1.
	\end{align*}
	
	Finally we get:
	$$
	\sigma^{(t)} = \sqrt{\text{Var}(x)} = \sqrt{p(t) \sigma_1^2(t) + \mu_1^2(t)(1-p(t)p(t)}.
	$$
\end{proof}

We now prove the Theorem \ref{theo:thresh_impr}
\begin{proof}{[Threshold increases probability] (intuition behind the proof)}

	Let's show that the theorem holds for some nontrivial case with moderate $t$. First, we notice that the terms in Lemma \ref{lem:concentration_bound} do not depend on permutations of the domain of $f_{\mathcal{R}}$, therefore for this analysis we can reorder the function according to decreasing values. Let's assume that $f_{\mathcal{R}}(x)$ can be approximated by an exponential law $f_{\mathcal{R}}(x) = \lambda e^{-\lambda x}$ (after reordering the values). Therefore, we can approximate each terms from lemma \ref{lem:concentration_bound}:
	\begin{equation*}
		p(t) = \frac{-\log{(t/\lambda})}{\lambda},
	\end{equation*}
	\begin{align*}
		\mu_1(t) &= \int_0^{p(t)} x \cdot \lambda e^{-\lambda x} dx \\ &= \frac{1}{\lambda} - \frac{t}{\lambda^2} + \frac{t \log(t/\lambda)}{\lambda^2},
	\end{align*}
	\begin{align*}
		\sigma_1(t) &= \int_0^{p(t)} x^2 \cdot \lambda e^{-\lambda x} - \mu^2\\ &= \frac{(\lambda^2 - t^2 + 2 t^2 \log[t/\lambda] - t (\lambda + t) \log[t/\lambda]^2)}{\lambda^4}.
	\end{align*}
	
	Putting everything together in Lemma \ref{lem:concentration_bound}, we obtain an explicit expression for the value $\sigma^{(t)^2}$. For a fixed $\lambda$, the function in $t$ increases before reaching a maximum and then decreases. One can also check $\lim_{t \rightarrow \infty} \sigma^{(t)^2} = 0$. Finally, since the function $f_\mathcal{R}$ is continuous, the Intermediate Value Theorem tells us that there exists a value of $t$ for which $\sigma^{(t)^2} \leq \sigma^2$. This end the proof of Theorem \ref{theo:thresh_impr}.    
\end{proof}

\newpage
\section{Intuition behind Algorithm 1}
\label{app:old_just}

In this Supplementary Information, we provide a heuristic justification of the algorithm supported by numerical simulation and rigorous proofs of lemmas and propositions whenever possible. We focus on a specific example and explain the detailed behavior of Alogirhtm 1.

Consider a simplified situation with a single 3-bit rule $r=r_1r_2r_3$. We define our target problem, which is to find a binary string $x^*_I$ that contains as many sub-string identical to $r$ as possible. Notice that $r$ is unknown and does not need to be known, while  $x^*_I$ is learned based on rewards given to randomly selected binary strings, where for a given string the reward is equal to the number of times the rule $r$ appears in it.  

In Algorithm 1, we solve {Problem II where the rows of matrix $\Phi$, are given by\\
	\noindent{\bf Duplets}
	\begin{eqnarray}
		\Phi^{i,i+1}_{x_1,x_2} &=&1_1\otimes … \otimes 1_{i-1}\label{eq:measur}\\
		&\otimes& (1-x_1,x_1)\otimes(1-x_2,x_2)\otimes 1_{i+2}\otimes…\otimes 1_N\nonumber
	\end{eqnarray}
	for the $[4(i-1)+2x_1+x_2+1]$-th row and $x_1$ and $x_2$ are binary variables.\\
	
	\noindent Define variable $\mu^i_x=\Phi^{i}_{x}Y$, where 
	$$\Phi^{i}_{x} = 1_1\otimes … \otimes 1_{i-1}\otimes (1-x,x)\otimes 1_{i+1}\otimes…\otimes 1_N$$ 
	is a \textbf{Singulet} map and
	$$Y = (1-y_1,y_1)\otimes … \otimes (1-y_n,y_n),$$ 
	is a vector whose entries are zero except at the position given by the binary variables $y_i\in\{0,1\}$.
	If vectors $Y$ are randomly chosen from a distribution, the variable $\mu^i_x$ is a random variable. Assume $Y$ are defined by arguments of the function $T_tSf_{\mathcal{R}}$---lines sampled uniformly from $f_{\mathcal{R}}$ and thresholded. 
	
	Moments $\varphi^{i,i+1}_{x_1,x_2}= \langle\mu^i_{x_1}\mu^{i+1}_{x_2}\rangle$ are calculated as $\Phi^{i,i+1}_{x_1,x_2} T_tSf_{\mathcal{R}}$, where
	$\Phi^{i,i+1}_{x_1,x_2}$ is given in (\ref{eq:measur}).
	Up to normalization, these moments express averages over sampled elements of $f_\mathcal{R}$ with weights corresponding to the value each element. Analogously, we consider moments $\varphi^{i,i+1,i+2}_{x_1,x_2,x_3}=\langle\mu^i_{x_1}\mu^{i+1}_{x_2}\mu^{i+2}_{x_3}\rangle$. These averages are related to appropriate correlation functions
	$$
	corr^{i_1...i_n}_{x_{i_1},...,x_{i_n}}=\frac{\langle(\mu^{i_1}_{x_{i_1}}-\langle\mu^{i_1}_{x_{i_1}}\rangle)...(\mu^{i_n}_{x_{i_n}}-\langle \mu^{i_n}_{x_{i_n}}\rangle)\rangle}{\langle\mu^{i_1}_{x_{i_1}}\rangle...\langle \mu^{i_n}_{x_{i_n}}\rangle}.
	$$
	Therefore, loosely speaking, the  moments express correlations between a given bit configuration $x_1...x_n \in \lbrace 0,1 \rbrace^n$ and the appearance of this configuration in important elements of the sample from $f_{\mathcal{R}}$. The importance is specified by values of $f_\mathcal{R}$ that remain after sampling and thresholding. 
	
	In Algorithm 1 we solve Problem II, which is, we find a string $x^*_{II}$ for which the sum of correlations for neighboring variables is maximized,
	\begin{equation}
		x^*_{II}=\argmax\sum_{i=1}^{N-1} \varphi^{i,i+1}_{x_1,x_2}.\label{eq:x2solu}
	\end{equation}
	Moreover, the way Algorithm 1 assigns the values $\varphi^{i,i+1}_{x_1,x_2}$ induces correlations between these values. 
	
	Our numerical analysis shows that solving Problem II often suffices to solve Problem I. Because $x^*_I$ contains several times $r_1r_2r_3$ it is true that $r_2$ follows $r_1$ more often than in a random string (the same for the pair $r_3$ and $r_2$), and obviously, $r_3$ follows the pair $r_1r_2$ more often than in random sequences. Therefore, the minimum requirement for any solver of Problem I should be to propose candidate solutions $x$ which: 
	\begin{itemize}
		\item Condition 1: possibly often contain pairs of bits $r_1r_2$ and $r_2r_3$, and
		\item Condition 2: the pairs appear in proper order, $r_2r_3$ likely appear after $r_1r_2$.
	\end{itemize}
	
	Notice that the solution of Problem II is a binary string $x^*_{II}$ which is defined by the lower indices of the variables $\mu^i_{x_i}$ for 
	which the sum of correlations $\varphi^{i,i+1}_{x_1,x_2}=\langle\mu^i_{x_1}\mu^{i+1}_{x_2}\rangle$ is maximum (as in Equation (\ref{eq:x2solu})).
	In the following proposition (proven in Supplementary Information \ref{app:prop1}), we claim that pairs of variables with $x_1x_2$ matching substrings of $r$ have larger expected moments than bits that does not match $r$. 
	
	\begin{proposition}\label{prop:Aii}
		Let $\varphi^{i,i+1}_{x}=\Phi^{i,i+1}_xf_{\mathcal R}$,
		\begin{enumerate}[label=(\roman*), ref=(\roman*)]
			\item for the problem with single rule  $r$, for any $2 \leq i \leq N-2$, if $r'$ is a substring of $r$, and  $z$  is not, then
			$$\varphi^{i,i+1}_{r'}  \geq  \varphi^{i,i+1}_{z},$$    
			\item    for the problem with single rule $r$, for any $i$, there exists at least one $r'$ substring of $r$ such that, for any string $ z $:
			$$
			\varphi^{i,i+1}_{r'}  \geq  \varphi^{i,i+1}_{z},
			$$
			\item for the problem with single rule $r$, for any $i$, there exists at least one $r'$ substring of $r$ such that, for any string $ z $ the expectation values $\langle \varphi^{i,i+1}_{r}\rangle=\Phi^{i,i+1}_xT_tSf_{\mathcal R}$ satisfy:
			
			$$
			\langle \varphi^{i,i+1}_{r'}\rangle  \geq  \langle \varphi^{i,i+1}_{z}\rangle.
			$$
		\end{enumerate}
	\end{proposition}
	
	Therefore, solvers of Problem II (like Algorithm 1) promotes outputs $x^*_{II}$ including substrings of $r$, hence Condition 1 is satisfied.
	Condition 2 is also expected in the output $x^*_{II}$ of Problem II solvers. This comes from the consistency of the bits in  $\varphi^{i,i+1}_{x_1,x_2}$ and $\varphi^{i+1,i+2}_{x_2,x_3}$ — in the correct ordering bit $x_2$ is shared. In the opposite order, $x_3$ and $x_1$ cannot always be shared, and the bits $x_3x_1$ may not be among preferred substrings of $r$. The right order is also expected based on the effect of thresholding. It guaranties that in all addresses of randomly selected lines of $f_{\mathcal{R}}$, if $r_1r_2 $ is found in position $i,i+1$ in any of the lines the probability that $r_3$ follows is high or increases with increasing threshold. This in turn is reflected in high values of both the correlation $\varphi^{i,i+1}_{x_1,x_2}$   and $\varphi^{i+1,i+2}_{x_2,x_3}$. The thresholding argument penalizes the incorrect order of the correlation functions. Moreover, it penalizes strings with repeated subsings $r_1r_2$ not followed by $r_3$.         
	
	Therefore, we argue that Algorithm 1 which formally solves Problem II satisfies the minimum requirements of solver of Problem I. Thus, the output $x_{II}^*$ of Algorithm 1 is also, with high probability, a solution of Problem I, as confirmed in the numerical simulations.
	
	The arguments presented here are focused on providing an understanding based on simplified assumptions including a single rule of size three. The generalization for multiple different rules which is still confirmed by the numerical tests is in many cases a complicated problem. The rigorous proof can go along the same line of reasoning. However, calculating related probabilities rigorously can require solving counting satisfying assignments of logical formulas which are $\#P$ problems. Computing upper and lower bounds on the success probability remains an open problem.
	
	\subsection{Proof of Proposition 1---Larger moments of substrings of the rules}\label{app:prop1}
	
	\begin{proof}
		Formally,
		$$
		\varphi^{i,i+1}_{x} = (\Phi^{i,i+1}_x)^T F_N(r),
		$$
		where
		$$
		\Phi^{i,i+1}_x = (1_1\otimes … \otimes 1_{i-1}\otimes x\otimes 1_{i+2}\otimes…\otimes 1_N)
		$$
		and
		$$
		F_N(r) = r \otimes 1_4\otimes …\otimes 1_N\\+1_1\otimes r \otimes 1_5\otimes …\otimes 1_N\\...\\+1_1\otimes …\otimes 1_{N-3}\otimes r.
		$$
		
		i) For any position $2 \leq i \leq N-2$, %refer to the proof of Proposition 1 (i)
		
		For a measurement bits $x_1x_2$ to match the rules at those positions, there are four possibilities shown in Table \ref{tab:t1}:\\
		
		\begin{table}[!b]
			\begin{tabular}{|c|c||c|c||c|c|}
				\hline
				. & . & $x_1$ & $x_2$ & . & . \\ \hline
				$r_1$ & $r_2$ & $r_3$ & . & . & . \\ \hline
				. & $r_1$ & $r_2$ & $r_3$ & . & . \\  \hline
				. & . & $r_1$ & $r_2$ & $r_3$ & . \\
				\hline
				. & . & . & $r_1$ & $r_2$ & $r_3$ \\ \hline
			\end{tabular}\caption{Configurations in which two bits $x_1$ and $x_2$ inside a string can mach the rule $r_1r_2r_3$.}
			\label{tab:t1} \end{table}
		
		\begin{itemize}
			\item If $x_1x_2$ matches either $r_1r_2$$r_1 r_2$$r_2 r_3$ → the energy increases by $2^{N-3}$
			\item If $x_1$ matches $r_3$ → the energy increases by $2^{N-4}$
			\item If $x_2$ matches $r_1$ → the energy increases by $2^{N-4}$
			\item Any other case → the energy increases by $0$
		\end{itemize}
		
		So in total, any sketching pattern that are substring of a rule ( $r_1r_2$ or $r_2 r_3$) will bring $2^{N-3}$ energy. The other most energetic case is $x_1x_2 = r_3 r_1$ which brings $2 \times 2^{N-4} = 2^{N-3}$ energy (same amount). 
		
		All other cases bring less energy. So we have indeed for all subtring $r$ and any $z$ $m^{i,i+1}_{r}  \geq  m^{i,i+1}_{z}$. If it’s true for all, then it’s also true for at least one.
		
		ii) We study matching at the beginning and at the end
		
		a) matching in position 1,2, (Table \ref{tab:t2}).
		
		\begin{table}[]
			\begin{tabular}{||c|c||c|c|c|c|}
				\hline
				$x_1$ & $x_2$ & . & . & . & . \\ \hline
				$r_1$ & $r_2$ & $r_3$ & . & . & . \\ \hline
				. & $r_1$ & $r_2$ & $r_3$ & . & . \\  \hline
				. & . & $r_1$ & $r_2$ & $r_3$ & . \\
				\hline
				. & . & . & $r_1$ & $r_2$ & $r_3$ \\ \hline
			\end{tabular}\caption{Configurations in which two bits $x_1$ and $x_2$ at the beginning of a string can mach the rule $r_1r_2r_3$.}
			\label{tab:t2} \end{table}
		
		\begin{itemize}
			\item If $x_1x_2$ match $r_1r_2$ → the energy increases by $2^{N-3}$
			\item If $x_2$ matches $r_1$ → the energy increases by $2^{N-4}$
			\item Any other case → the energy increases by 0
		\end{itemize}
		So there is one substring $r$ , namely $r_1 r_2$, that brings more energy than any other string.
		
		The other substring all bring $0$ energy for this position.
		
		b) matching in position N-1,N (Table \ref{tab:t3}).
		
		\begin{table}[]
			\begin{tabular}{|c|c|c|c||c|c||}
				\hline
				.&.&.&.&$x_1$ & $x_2$ \\ \hline
				$r_1$ & $r_2$ & $r_3$ & . & . & . \\ \hline
				. & $r_1$ & $r_2$ & $r_3$ & . & . \\  \hline
				. & . & $r_1$ & $r_2$ & $r_3$ & . \\
				\hline
				. & . & . & $r_1$ & $r_2$ & $r_3$ \\ \hline
			\end{tabular}\caption{Configurations in which two bits $x_1$ and $x_2$ at the end of a string can mach the rule $r_1r_2r_3$.}
			\label{tab:t3} \end{table}
		
		\begin{itemize}
			\item If $x_xm_2$ match $r_2r_3$ → the energy increases by $2^{N-3}$
			\item If $x_1$ matches $r_3$ → the energy increases by $2^{N-4}$
			\item Any other case → the energy increases by $0$
		\end{itemize}
		
		So there is one substring $r$ , namely $r_2 r_3$, that brings more energy than any other string.
		
		The other substring all bring $0$ energy for this position.
		
		Part (iii) easily follows from (ii).
	\end{proof}
	
	For the problems with multiple rules the above reasoning should be completed by multiplying powers of two by appropriate factors proportional to values of rewards. The statements regarding the ordering of  $<\varphi^{i,i+1}_{x}>$ for x belonging to different rules, or appearing in different rules, or not belonging to any of them is more complicated. However, similar arguments to Propositions \ref{prop:Aii} supported by numerical simulations allow us to conjecture that Algorithm 1 assigns higher values $\langle \varphi^{i,i+1}_{x}\rangle$ to pairs of bits $x$ which are parts of the rules.

\end{document}
